# Supplementary material for: Nested Papercrafts for Anatomical and Biological Edutainment
Source: arXiv:2204.10901 source file (2022-04-22)
Supplement: Supplementary file 1 [file 8-appendix.tex]

% \appendix
% \renewcommand{\thesection}{\Alph{section}.\arabic{subsection}}

\setcounter{section}{0}

\section*{Supplementary Material}
\label{sec:appendix}

In the appendix, we provide the unfolded patches of Figure~\ref{fig:teaser} (c) with better image resolution. 
\rv{Our readers} can print them out and build their own head papercraft.
First of all, the \rv{three} pages need to be printed double-sided with long-edge binding.
It is recommended to print on A3 paper or other larger formats.
Once the patches are printed, they need to be cut out. 
Before reconstruction, it is recommended to bend the triangles on the solid lines and observe the patches in advance.
Once everything is prepared, double-sided tape to the glue tabs can be applied.
Then, the numbers on the glue tabs need to be matched with the numbers on the matching area on the back side of the paper. 
We recommend to start with the last page that contains the smallest structure (i.e., the brain).
The other two include the two halves of the skull. 
After the papercraft is built, the projected structures can be investigated with colored filters (i.e., simple colored foils) or under colored light (red, green, blue). 
Enjoy!

\section{The Head Dataset}
\label{app:head1}
\clearpage
\includepdf[pages={-}, angle=0]{appendix/print_head_userstudy_new.pdf}
